# Supplementary material for: An Effective Transition-based Model for Discontinuous NER
Source: arXiv:2004.13454 source file (2020-04-28)
Supplement: Supplementary file 1 [file appendix.tex]

\subsection{Contributions of Attention and Pretrained Word Representations}

\begin{table}[t]
\begin{small}
\setlength{\tabcolsep}{4pt} % Default value: 6pt
    \centering
    \begin{tabular}{ lc  c c c c c}
    \toprule
    && \multicolumn{2}{c}{\bf CADEC} && \multicolumn{2}{c}{\bf ShARe 2013} \\ \cmidrule{3-4}\cmidrule{6-7}
    \bf Model&& All & w. Disc. && All & w. Disc. \\ \cmidrule{1-1}\cmidrule{3-4}\cmidrule{6-7}
    Full && \bf 68.4 & \bf 65.4 && \bf 77.2 &  \bf 64.3 \\ 
    -Attention && 68.4 & 63.3 && 76.8 & 62.3 \\ 
    - ELMo && 66.7 & 62.2 && 75.2 & 60.9 \\ 
    BERT && 67.2 & 64.4 && 73.7 & 59.3 \\ \bottomrule
    \end{tabular}
    \caption{Ablation study to estimate the contribution of attention and pretrained contextual representations.~\label{table4-ablation}}
\end{small}
\end{table}

To empirically evaluate the importance of attention and ELMo components, we test the performance of model variants where attention and ELMo are removed separately on CADEC and ShARe 2013 data sets. In addition, we evaluate one variant built on top of BERT encoder. More specifically, we replace $\mathbf{c_i}$ in Equation~\ref{equ:elmo} as the output from BERT, and keep the BERT encoder trainable.

The results in Table~\ref{table4-ablation} show that removing attention hurts the performance when evaluated on sentences with discontinuous mentions (\textit{w. Disc.} columns), but have little impact on the complete test set where continuous mentions are prevalent. Since we use BiLSTM to derive contextual representation for each token, we believe these contextual representations are effective at recognizing continuous mentions, but have trouble identifying intervals within discontinuous mentions. Attention mechanism, via allowing tokens interacting with distant tokens, can capture additional discontinuous dependencies which are not captured by BiLSTM.

In terms of pretrained word representations, on one hand, we find that ELMo component contributes approximately two $F_1$ score when evaluated on the complete test set and around four $F_1$ when evaluated on sentences with discontinuous mentions, demonstrating the usefulness of pretrained word representations. On the other hand, BERT does not achieve as good performance as ELMo (even worse on ShARe 2013 than the model variant without ELMo component). We hypothesize this could be caused by different adaptation strategies used by ELMo and BERT. That is, the \emph{feature extraction approach} used by ELMo enables more complex task-specific architecture whereas \emph{fine-tuning approach} used by BERT may provide a more convenient general-purpose architecture.

\subsection{Training on more balanced data set}
The three data sets we use are all very imbalance regarding the number of discontinuous and continuous mentions. 
Only around 10\% of mentions are discontinuous.
To evaluate the performance of our model trained on more discontinuous mentions, we experimented with three additional settings on ShARe 2013 data set, inspired by~\cite{Muis:Lu:EMNLP:2016}.
\begin{enumerate}[I]
    \item Training only on sentences that contain discontinuous mentions;
    \item Training on a balanced data set by under-sampling sentences without discontinuous mentions;
    \item Training on a balanced data set by over-sampling sentences with discontinuous mentions.
\end{enumerate}
The test set is kept unchanged.

Our model can achieve higher performance on recognizing discontinuous entities when it is trained on more discontinuous mentions (See the last row in Table~\ref{table:balance-dataset}). However, similar to other neural-based models, the performance substantially decreases when the training data is limited. 

\begin{table}[]
\begin{small}
    \centering
    \begin{tabular}{c|c|c|c}
    \toprule
    & \makecell{\# Training \\ sentences} & All & w. Disc. \\ \hline
    Original training set & 9758 & \textbf{77.2} & 60.2 \\ 
    \cite{Muis:Lu:EMNLP:2016} & -- & -- & 54.3 \\
    \Romannum{1} & 536 & 33.6 & 54.6 \\
    \Romannum{2} & 1005 & 53.7 & 58.3 \\
    \Romannum{3} & 18334 & 73.0 & \textbf{63.4} \\
    \bottomrule
    \end{tabular}
    \caption{The $F_1$ score evaluated on ShARe 2013 test set of our model trained on more balanced data set regarding the number of discontinuous and continuous mentions. Result of~\cite{Muis:Lu:EMNLP:2016} is taken from the original paper, which is trained on only sentences that contain discontinuous mentions (our setting \Romannum{1}). ~\label{table:balance-dataset}}
\end{small}
\end{table}

\subsection{Effectiveness of Our Model on Flat NER Data Sets}
Our model can be directly applied on data set with only continuous mentions.
To evaluate the effectiveness of our model on these flat entity mentions that are usually short spans of text, we run experiments on a widely used NER data set: CoNLL2003. 
Our model achieves competitive results (89.7 $F_1$ score versus 90.2 $F_1$ score of the BiLSTM-CRF model). Note that the only external resource we use in both experiments are GloVe pretrained word vectors~\cite{Pennington:Socher:EMNLP:2014}.
